# Supplementary material for: Naturally Rehearsing Passwords
Source: arXiv:1302.5122 source file (2013-09-09)
Supplement: Supplementary file 1 [file AppendixBaselineSchemes.tex]

\section{Example Password Management Schemes} \label{sec:ExamplePasswordManagementSchemes}

\begin{enumerate}
\item \ReuseWeakPassword: $\Generator\paren{k,b}$ selects $w \in D_{20,000}$ uniformly at random, and sets $p_i = w$ and $c_i = \emptyset$ for all accounts $i$.    
\item  \ReuseStrongPassword: $\Generator\paren{k,b}$ independently selects four words $w_1,w_2,w_3,w_4 \in D_{20,000}$ uniformly at random, and sets $p_i = w_1w_2w_3w_4$ and $c_i = \emptyset$ for all accounts $i$. 
\item \Lifehacker (e.g., \cite{guideline:lifehacker}): $\Generator\paren{k,b}$ selects a base password $b = w_1w_2w_3$ by selecting $w_1,w_2,w_3 \in D_{20,000}$ independently at random. $\Generator\paren{k,b}$ also derivation rule $d$ uniformly at random from a set of 50 simple derivation rules (e.g., use the first three letters of the account name $A_i$, use the first three vowels in the account name). Finally, $p_i = w_1w_2w_3\#d(A_i)$ and $c_i = \emptyset$. 
%\item {\bf NIST:} The user picks a base password $b = w_1w_2w_3$ by selecting $w_1,w_2,w_3 \in D$ independently at random. For each account $i$ the user selects three random alphanumeric characters $y^i_1,y^i_2,y^i_3$ independently at random, and sets $p_i = w_1y^i_1w_2y^i_2w_3y^i_3$  $c_i$ and $r_i$ are the empty cue and the blank rehearsal schedule respectively. This password management scheme is similar in nature to the informal suggestions given by NIST \cite{guideline:NIST2009}.
\item {\StrongRandomPassword:} For each account $i$ $\Generator\paren{k,b}$ selects four words $w_1^i,w_2^i,w_3^i,w_4^i \in D_{20,000}$ uniformly at random and sets $p_i =  w_1^iw_2^iw_3^iw_4^i$ and $c_i = \emptyset$. 
\end{enumerate}

We formally analyze the security and usability of each of these schemes in the appendix. We find that the first three schemes (\ReuseWeakPassword,\ReuseStrongPassword,\Lifehacker) are easy to use, but only satisfy weak security guarantees. \StrongRandomPassword provides very strong security guarantees, but is highly difficult to use. In section \ref{sec:PicturesAsCues} we present our password management scheme: \sharedCues. We demonstrate that \sharedCues satisfies strong security properties and is almost as easy to use as \ReuseStrongPassword.
